# Supplementary material for: The Media Bias Taxonomy: A Systematic Literature Review on the Forms and Automated Detection of Media Bias
Source: arXiv:2312.16148 source file (2024-01-10)
Supplement: Supplementary file 1 [file Appendix_old.tex]

% For example, not every statement containing the word \textit{murder} is biased (cf. ``He was convicted of murder'' \cite{Hube_2018b}). However, depending on the context, \textit{murder} becomes an indicator for bias (cf. ``An abortion is the murder of a human baby'' \cite{Hube_2018b} vs. ``An abortion is the intentional ending of a pregnancy''\footnote{https://dictionary.cambridge.org/us/dictionary/english/abortion; accessed on 2022-02-25})

%For example, gun owners are more likely to perceive an article about a stronger gun control law as hostile towards their point of view because they are emotionally more involved than non-gun owners \cite{Zhang_2021}

%For example, news stories published by Fox News are generally perceived to be biased towards Republican's point of view \cite{Baum_2008}.

%For example, presenting readers an article where biased sentences are marked improves the reader's awareness about that bias.

%While women occur more in articles with the topics lifestyle, entertainment, and healthcare, men are more present in articles with topics such as business, politics, and sports \cite{rao2021gender}

\section{Appendices} \label{sec:appendix}

%Table 1/2 Table 2. Bias Overview
\begin{table*}[!htp]
\centering
\resizebox{0.999\textwidth}{!}{
  \begin{tabular}{p{0.15\textwidth}P{0.19\textwidth}P{0.14\textwidth}p{0.27\textwidth}P{0.08\textwidth}P{0.25\textwidth}}
    \toprule
    Bias Category&Subcategory&Features&Definition&Source&Example\\
    \midrule
    Linguistic Bias & & & & & \\
    \midrule
     & Framing Bias
     & 
     & Subjective words or phrases linked with a certain point of view.
     & \citep{recasens-etal-2013-linguistic} 
     & Usually, smaller cottage-style houses have been demolished to make way for these \textbf{\textit{McMansions}}.
     \\\addlinespace[0.3cm]
     %
     &
     & Subjectivity Clues
     & Subjectivity clues are words which in most (\textit{strongsubj}) or certain (\textit{weaksubj}) contexts are considered to add subjective meaning to a statement.
     & \citep{riloff-wiebe-2003-learning, wilson-et-al2005recognizing}
     & Subjective adjectives (e.g., preposterous, unseemly) and metaphorical or idiomatic phrases(e.g., dealt a blow, swept off one’s feet).
     \\\addlinespace[0.2cm]
     %
     & 
     & One-sided Terms
     & One-sided terms only reflect on one side of a controversial subject where the same event can be seen from two or more opposing perspectives.
     & \citep{recasens-etal-2013-linguistic}
     & "\textbf{\textit{Pro-life}}" vs. "anti-abortion".
     \\\addlinespace[0.2cm]
     %
     & Epistemological Bias
     & 
     & Linguistic features that subtly focus on the believably of a position.
     & \citep{recasens-etal-2013-linguistic}
     & Kuypers \textbf{\textit{claimed}} that the mainstream press in America tends to favor liberal viewpoints.
     \\[13pt]
     %
     & 
     & Factive Verbs
     & Factive verbs presuppose the truth of a complement clause.
     & \citep{hooper1975on, karttunen1971implicative}
     & "John \textbf{\textit{realized}} that he had no money" implies "John had no money".
     \\\addlinespace[0.2cm]
     %
     & 
     & Entailments
     & Entailments are directional relations where one statement implies the truth of another.
     & \citep{berant-etal-2012-efficient, karttunen1971implicative}
     & “Cyprus \textbf{\textit{was invaded by}} the Ottoman Empire in 1571” implies the hypothesis “The \textbf{\textit{Ottomans attacked}} Cyprus”.
     \\\addlinespace[0.2cm]
     %
     & 
     & Assertive Verbs
     & Assertives imply that the speaker or subject of a sentence has an affirmative opinion on the truth value of a complements proposition.
     & \citep{hooper1975on}
     & E.g. regret, resent, forget, amuse, suffice, bother.
     \\\addlinespace[0.2cm]
     %
     & 
     & Hedge Words
     & Hedge words are used to lessen the probability and the writer's guarantee of truthfulness of a statement.
     & \citep{hyland2005metadiscourse}
     & E.g. perhaps, might, may.
     \\\addlinespace[0.2cm]
     %
     & Bias by Semantic Properties
     & 
     & A set of semantic properties which are grammatically relevant and serve as an interface between syntax and semantics.
     & \citep{greene-resnik-2009-words}
     & "The gunmen shot the opposition leader" vs. "The shooting killed the opposition leader".
     \\\addlinespace[0.2cm]
     %
     & 
     & Causative-Inchoative Alternations
     & Causative-inchoative alternations are verbs that can either emphasize a change of state or the bringing about of the change of state.
     & \citep{greene-resnik-2009-words, Pin2001AFL, Levin1993} 
     & "Rebecca broke the pencil" vs. "The pencil broke".
     \\\addlinespace[0.2cm]
     %
     & Connotation Bias
     & 
     & Bias through the use of different words for the same subject with identical denotations but differing (often biased) connotations.
     & \citep{webson-etal-2020-undocumented, chakrabarty2021entrust} 
     & E.g. “immigrants” vs. “\textbf{\textit{aliens}}”, “estate tax” vs. “\textbf{\textit{death tax}}”.
     \\\addlinespace[0.2cm]
     %
     & 
     & Verb Connotations
     & Verbs with identical denotation but differing connotation.
     & \citep{rashkin-etal-2016-connotation}
     & The story begins in Illinois in 1987, when a 17- year-old girl \textbf{\textit{suffered}} a botched abortion.
    \\\addlinespace[0.2cm]
    %
%    & 
%    & Noun and Adjective Connotations
%    & Nouns and adjectives with identical denotation but differing connoations.
%    & \citep{allaway2021unified}&relentless (-) vs. persistent (+)     gentleman (+) vs. man (=) protection (-)      vs. security (=)\\\addlinespace[0.2cm]
%    & Linguistic Intergroup Bias& & Variations in language that lead to the creation or maintenance of                  reputations of certain social groups.& \citep{dragojevic2017evidence} &"Mary hit Mike" vs. "Mary hurt            Mike" vs. "Mary hates Mike" vs. "Mary is aggressive"
%    \\\addlinespace[0.2cm]
    \end{tabular}
}    
\caption{Bias Overview} 
\label{table:categories1}
\end{table*}

%---------------------------------------------------------------------
%Table 2/2 Table 2. Linguistic Bias 
%---------------------------------------------------------------------
\begin{table*}[!htp]
\centering
\resizebox{0.999\textwidth}{!}{
  \begin{tabular}{p{0.15\textwidth}P{0.19\textwidth}P{0.14\textwidth}p{0.27\textwidth}P{0.08\textwidth}P{0.25\textwidth}}
    \toprule
    Bias Category&Subcategory&Features&Definition&Source&Example\\
    \midrule
    Linguistic Bias & & & & & \\
    \midrule
    %
     &% Connotation Bias
     & Noun and Adjective Connotations
     & Nouns and adjectives with identical denotation but differing connotations.
     & \citep{allaway2021unified} 
     & relentless (-) vs. persistent (+) gentleman (+) vs. man (=) protection (-) vs. security (=)
    \\\addlinespace[0.2cm]
     % 
     & Linguistic Intergroup Bias 
     & 
     & Variations in language that lead to the creation or maintenance of reputations of certain social groups. 
     & \citep{dragojevic2017evidence}
     & "Mary hit Mike" vs. "Mary hurt Mike" vs. "Mary hates Mike" vs. "Mary is aggressive".
    \\\addlinespace[0.2cm]
% ------------------------------------------------------------------------------------------------------
%
%Ab hier allen Content aus der Table entfernen
%-------------------------------------------------------------------------------------------------------
     & 
     & 
     & 
     & A set of semantic properties which are grammatically relevant and serve as an interface between syntax and semantics.
     & 
     &"The gunmen shot the opposition leader" vs. "The shooting killed the opposition leader"
    \\\addlinespace[0.2cm]
%
     & 
     & Causative-inchoative alternations are verbs that can either emphasize a change of state or the bringing about of the change of state.
     & \citep{greene-resnik-2009-words, Pin2001AFL, Levin1993} 
     &"Rebecca broke the pencil" vs. "The pencil broke"
     &
    \\\addlinespace[0.2cm]
%
    & 
    & 
    & \citep{allaway2021unified}
    & relentless (-) vs. persistent (+)  gentleman (+) vs. man (=) protection (-) vs. security (=) 
    &
    \\\addlinespace[0.2cm]
    \end{tabular}
}    
\caption{Bias Overview 2} 
\label{table:categories12}
\end{table*}

%---------------------------------------------------------------------
%Table Context Bias (Text Level)
%---------------------------------------------------------------------
\begin{table*}[!htp]
\centering
\resizebox{0.999\textwidth}{!}{
    \begin{tabular}{p{0.15\textwidth}P{0.19\textwidth}P{0.17\textwidth}p{0.25\textwidth}P{0.08\textwidth}P{0.25\textwidth}}
    \toprule
    Bias Category&Subcategory&Features&Definition&Source&Example\\
    \toprule
    \raggedright{Context Bias (Text Level)}& & & & &\\
     \midrule
     & Spin Bias
     & 
     & Emerges through a newspaper’s attempt to create a memorable story by means of simplification or exaggeration. In the case of simplification, newspaper discard some information, whereas exaggeration shapes the story towards a certain direction. Both methods try to present the news in a way to attract potential readers.
     & \citep{mullainathan2002media, alsem2008impact}
     &President Donald Trump \textbf{\textit{gloated}} over mass layoffs at multiple news outlets on Saturday.
     \\\addlinespace[0.2cm]
     %
     & Statement Bias
     & 
     & Refers to the process how facts are reported. This can be by means of expressing own opinions, criticizing the counterpart, or advocating the own viewpoints in a way that news reporting is favorable or unfavorable towards a certain standpoint.
     & \citep{dalessio-et-al2006media}
     &A political protest in which people sat down in the middle of a street blocking traffic can be described as “peaceful” and “productive,” or, others may describe it as “aggressive” and “disruptive"
     \\\addlinespace[0.2cm]
     %
     & Omission Bias / Commission Bias
     & 
     & Omission or Commission Bias results from the journalists' decision of what (substantial) information to exclude and what information to include in the news report.
     & \citep{martinez-alonso-etal-2017-annotating, hamborg2019automated}
     &CNN previously reported on the FBI's hate crime statistics released last November, which showed the number of hate crimes reported to the bureau rose about 17\% in 2017 compared to 2016. 2017 is the latest year for which those statistics are available. It was the third-straight year that hate crime incidents rose.
     \\\addlinespace[0.2cm]
     %
     & Informational Bias
     & 
     & A statement containing Informational Bias serves to purpose to influence the readers’ opinion. This may be done by adding information, which is not necessarily relevant to the event or rather speculative.
     & \citep{fan2019a}
     &Often embedded in context, see \citep{fan2019a}
     \\\addlinespace[0.2cm]
     %
     & Phrasing Bias
     & 
     & Phrasing Bias results from using words in a sentence or statement which are inflammatory or partial.
     & \citep{hube2019a}
     & "aborting the fetus" vs. "killing the baby"\\\addlinespace[0.2cm]
     
     
     \raggedright{Context Bias (Reporting Level)}& & & & &\\[13pt]
     \midrule
     %
     & Coverage Bias
     & 
     & Coverage bias is concerned with the different amounts of coverage diverse sides of the same issue receive.
     & \citep{dalessio-et-al2006media}
     &A candidate of a political party receiving more coverage than the candidate of the other party.
     \\\addlinespace[0.2cm]
     & Selection Bias& & Selection bias occurs because of individuals in the news media being biased in their selection of events to report on.& \citep{dalessio-et-al2006media}&During the Roosevelt administration, the entire press was hostile against it in some parts of the country and it was impossible to get the other side of the story. 
     \\\addlinespace[0.2cm]
    \end{tabular}
}    
\caption{Bias Overview} 
\label{table:categories2}
\end{table*}


\begin{table*}[!htp]
\centering
\resizebox{0.999\textwidth}{!}{
    \begin{tabular}{p{0.15\textwidth}P{0.19\textwidth}P{0.17\textwidth}p{0.25\textwidth}P{0.08\textwidth}P{0.25\textwidth}}
    \toprule
    Bias Category&Subcategory&Features&Definition&Source&Example\\
    \toprule
    \raggedright{Context Bias (Text Level)}& & & & &\\
     \midrule
     & Spin Bias
     & 
     & Emerges through a newspaper’s attempt to create a memorable story by means of simplification or exaggeration. In the case of simplification, newspaper discard some information, whereas exaggeration shapes the story towards a certain direction. Both methods try to present the news in a way to attract potential readers.
     & \citep{mullainathan2002media, alsem2008impact}
     &President Donald Trump \textbf{\textit{gloated}} over mass layoffs at multiple news outlets on Saturday.
     \\\addlinespace[0.2cm]
     %
     & Statement Bias
     & 
     & Refers to the process how facts are reported. This can be by means of expressing own opinions, criticizing the counterpart, or advocating the own viewpoints in a way that news reporting is favorable or unfavorable towards a certain standpoint.
     & \citep{dalessio-et-al2006media}&A political protest in which people sat down in the middle of a street blocking traffic can be described as “peaceful” and “productive,” or, others may describe it as “aggressive” and “disruptive"
     \\\addlinespace[0.2cm]
     %
     & Omission Bias / Commission Bias
     & 
     & Omission or Commission Bias results from the journalists' decision of what (substantial) information to exclude and what information to include in the news report.
     & \citep{martinez-alonso-etal-2017-annotating, hamborg2019automated}
     &CNN previously reported on the FBI's hate crime statistics released last November, which showed the number of hate crimes reported to the bureau rose about 17\% in 2017 compared to 2016. 2017 is the latest year for which those statistics are available. It was the third-straight year that hate crime incidents rose.
     \\\addlinespace[0.2cm]
     %
     & Informational Bias
     & 
     & A statement containing Informational Bias serves to purpose to influence the readers’ opinion. This may be done by adding information, which is not necessarily relevant to the event or rather speculative.
     & \citep{fan2019a}
     &Often embedded in context, see \citep{fan2019a}
     \\\addlinespace[0.2cm]
     %
     & Phrasing Bias
     & 
     & Phrasing Bias results from using words in a sentence or statement which are inflammatory or partial.
     & \citep{hube2019a}
     & "aborting the fetus" vs. "killing the baby"
     \\\addlinespace[0.2cm]
     %
     \raggedright{Context Bias (Reporting Level)}& & & & &\\[13pt]
     \midrule
     & Coverage Bias
     & 
     & Coverage bias is concerned with the different amounts of coverage diverse sides of the same issue receive.
     & \citep{dalessio-et-al2006media}
     & A candidate of a political party receiving more coverage than the candidate of the other party.
     \\\addlinespace[0.2cm]
     %
     & Selection Bias
     & 
     & Selection bias occurs because of individuals in the news media being biased in their selection of events to report on.
     & \citep{dalessio-et-al2006media}
     & During the Roosevelt administration, the entire press was hostile against it in some parts of the country and it was impossible to get the other side of the story. 
     \\\addlinespace[0.2cm]
    \end{tabular}
}    
\caption{Bias Overview} 
\label{table:categories2}
\end{table*}


\pagebreak
\begin{table*}[!htp]
\resizebox{0.999\textwidth}{!}{
    \begin{tabular}{p{0.15\textwidth}P{0.19\textwidth}P{0.17\textwidth}p{0.25\textwidth}P{0.08\textwidth}P{0.25\textwidth}}
    \toprule
    Bias Category&Subcategory&Features&Definition&Source&Example\\
    \toprule
     \raggedright{Perception Bias}& & & & &\\
     \midrule
     & Political Ideology
     & 
     & Political Ideology determines the likelihood of a news consumer to perceive media as biased and influences what news sources are viewed as biased.
     & \citep{glynn2014how, lee2005liberal}
     &  Viewers of Fox News held distinct set of attitudes towards President George W. Bush (i.e., more favorable) as to his political opponents (i.e., less favorable) \citep{glynn2014how}.
     \\\addlinespace[0.2cm]
     %
     & Hostile Media Effect
     & 
     & The tendency of partisans to view media coverage as negative towards their own positions. Partisans also fear that nonpartisans could be swayed into a hostile direction by the media coverage.
     & \citep{vallone-et-al1985hostile, reid2012self-categorization, guntherschitt2004mapping, guntherliebhardt206broad, schmitt-et-al2004why, dalton-et-al1998american, Spinde2021-05Autom-52980}
     & Both Pro-Arab and pro-Israeli subjects seeing a US news programs on the  Israeli move into West Beirut as biased in favor of the other side.
     \\\addlinespace[0.2cm]
     %
     & Interpersonal Factors
     & 
     & Interpersonal Factors (e.g., ideological similarity) are related to the perception of media bias. 
     & \citep{eveland2003impact, CastroHopmannNir+2020}
     & Conversations with ideologically like-minded others increases the readers likelihood to perceive media as biased.
     \\\addlinespace[0.2cm]
     %
     & Article Comments
     & 
     & A news consumer being exposed to other users comments may influence the readers’ perception of this article being biased. Research shows that specifically those individuals who are confronted with incongruent opinions are likely to perceive stronger levels of media bias.& \citep{houston2003influence, lee2012thats, gearhart2020hostile}
     & Readers who saw a neutral Facebook post of an article on abortion with comments in line with their opinion perceived the story, writer, and outlet as less biased against their opinion.
     \\\addlinespace[0.2cm]
     %
     & Exposure to Opposing Views
     & 
     & Constant exposure to messages with opposing views from politicians and opinions leaders leads media consumers to perceive more bias in news media.
     & \citep{Bail9216}
     & Republicans who followed Twitter bots that retweeted liberal content exhibited more conservative views after one month of exposure.
     \\\addlinespace[0.2cm]
     %
     & Topic Identification / Involvedness
     & 
     & High involvement or identification with a topic or an issue are a reason of consumers' perception of media to be biased.
     & \citep{zhang2021effects, glynn2014how}
     & Persons who strongly identified with the republican party and were pro gun ownership perceived media bias in mass shooting news against gun owners to a higher degree.
     \\\addlinespace[0.2cm]
     %
     & Outlet Reputation
     & 
     & Reputation of media outlets ideological orientation can lead consumers to perceive bias in balanced news.
     & \citep{baum2008intheeye}
     & The perception of bias in the same news article depended on the brand or outlet name (e.g. CNN or FOX) study participants saw.
     \\\addlinespace[0.2cm]
  \bottomrule
\end{tabular}
}
\caption{Bias Overview} 
\label{table:categories3}

\end{table*}
